# Supplementary material for: Data-Driven but Privacy-Conscious: Pedestrian Dataset De-identification via Full-Body Person Synthesis
Source: arXiv:2306.11710 source file (2023-06-22)
Supplement: Supplementary file 1 [file supp.tex]

% 1) general task, evaluation metric - general stuff

% 2) \methodname details, SMPL

% 2-3) predicted masks, face anony

% 3) \methodname17. evaluation details

% 4) limitations and failure cases

% 5) qualitative results

\section{Pedestrian dataset de-identification}

\label{app_sec:imp_details}

% \noindent \textbf{Re-identification.}
% \paragraph{Re-identification.}
%
% \lau{Re-identification instead measures how well we can identify a person throughout a trajectory, providing a measure of stability of the generated identity.}
%
% For reID, we train a ResNet-50~\cite{he2016deep} backbone with cross-entropy loss and evaluate in a common single-shot-gallery setting.
% , \ie, randomly selecting one gallery and $N$ query samples for each identity in the cross validation set.
% in the MOT17~\cite{MOT16} training set .
%
% The random sampling provides a set of identification scenarios varying in their difficulty depending on the frame distance in the sequence.
% from adjacent frames.
%
% Furthermore, we only consider object instances with a visibility larger than zero and remove their background if MOTS20~\cite{MOTS} ground truth masks are available.

%
%Since we are anonymizing with partially predicted masks, we do not remove the background when evaluating deID.
%
%This allows us to measure the impact of undetected and therefore not de-identified object parts on the deID performance.

%

%
% reID
%
\subsection{Tasks}
\noindent \textbf{De- and re-identfication}
We evaluate a query-gallery experiment where both sets contain every annotated pedestrian identity.
This ensures we evaluate the de-identification quality for every person and all their occurrences in the dataset.
% de-identify all queries but refrain from random selection and add all samples to the gallery and query instead.
%
The deID performance is measured in a reverse re-identification experiment where we de-identify the query set and penalize the identification with any of their corresponding original gallery samples.
% , we consider  high de-identification performance is achieved by identifying the original instead of de-identified gallery samples.

% \noindent \textbf{De- and re-identfication.}
%
For both identification experiments, we apply a ResNet-50~\cite{he2016deep} feature extractor trained with a softmax cross-entropy loss.
The de- and re-identification performance is reported via CMC rank-1.
For each MOT17 sequence, the query-gallery sets are constructed and evaluated individually.
The MOT17 dataset contains annotations for fully occluded objects which can not be reasonably de- or re-identified, hence, we ignore all object instances with zero visibility.
We perform all de-identification evaluations with a model trained on the Market-1501~\cite{zheng2015scalable} dataset.

We evaluate the re-identification experiments in a single-shot-gallery setting, \ie, we randomly select one gallery and $N=5$ query samples for each identity in the cross-validation set. 
The random sampling provides a set of identification scenarios varying in their difficulty depending on the frame distance in the sequence.
Furthermore, we ignore tracks with less than 10 samples and objects with height/width smaller than 50/25 pixels.
Each split is trained for 40 epochs with a starting learning rate of 0.0001, which is then dropped by 0.1 every 10 epochs.
For both the training and validations sets, we remove the background of each person with the same set of masks as used for the de-identification.
This avoids potential identifications via similar backgrounds and ensures that the measured reID performance is only based on appearance features generated by the de-identification method.

%
% obj detection
%
\noindent \textbf{Object detection}
As an integral part of any tracking-by-detection MOT pipeline, we evaluate the performance of several object detectors.
% trained on the de-identified MOT17~\cite{MOT16} splits.
% pedestrian detection data, \ie, .
%
We train Faster R-CNN~\cite{rennips2015} (FRCNN) and RetinaNet~\cite{lin2017focal} with a ResNet-50 backbone, as examples of single-stage and two-stage detectors.

% \noindent \textbf{Object detection.}
For pedestrian detection, we train only on object instances with a visibility larger than 0.25 and evaluate on the official MOT17Det~\cite{lin2017focal} setup.
Consequently, the predicted and ground truth objects are matched with an intersection-over-union threshold of 0.5, while objects with visibility less than 0.5 are ignored.
For all experiments, we apply a ResNet-50 backbone and refrain from training its first two layers.
If trained from scratch, we apply a learning rate of 0.001 and batch size of 4 for 15 epochs.
For models pretrained on COCO~\cite{COCO} or MOTSynth, we fine-tune for 10 epochs with learning rates of 0.00004 and 0.0001 for the Faster R-CNN~\cite{rennips2015} and RetinaNet~\cite{lin2017focal} models, respectively.

\noindent \textbf{Multi-object tracking}
We evaluate the tracking performance of several state-of-the-art methods.
%
% The selected trackers differ in their reliance on spatial and/or appearance information.
%
The MOT performance is reported on the popular Tracktor~\cite{tracktor}, Tracktor with reID and CenterTrack~\cite{center_track} methods.
The selected methods represent different tracking approaches relying more or less on spatial and/or appearance information.
We train the trackers, and their underlying object detectors, on the de-identified data.

% \noindent \textbf{Multi-object tracking.}
For the Tracktor~\cite{tracktor} experiments, we apply the models obtained from the re-identification and Faster R-CNN trainings.
We evaluate with the default tracking settings and only adjust the detection and regression thresholds from 0.5 to 0.9.
This is due to a different training setup of the Faster R-CNN model compared to the original Tracktor model.
The CenterTrack models are trained and evaluated with track rebirth and default settings as in~\cite{center_track}.
Only for the model pretrained on MOTSynth, we apply a reduced learning rate of 0.0000125 for 30 epochs.
This fine-tuning learning rate is 10 times smaller as the one proposed by the authors.
However, we found this to work better for the MOTSynth model.

\subsection{Metrics}

    Each of the presented tasks is evaluated with a different set of metrics.
    For tracking, we follow the CLEAR MOT~\cite{clear_mot} evaluation metrics as implemented by MOT17.
    We present an overview and small description of each metric: 
    \begin{enumerate}[align=parleft, labelwidth=5em, labelindent=16pt, leftmargin=60pt]
    % \begin{enumerate}
        \item[CMC:] Cumulative Matching Characteristics (CMC) averages the number of positively matched re-identification queries in the top-$k$ gallery samples.
        \item[AP:] Detection Average Precision (AP) taken over a set of reference recall values (0:0.1:1).
        \item[MOTA:] Multi-Object Tracking Accuracy (MOTA) measuring object coverage by combining three error sources: false positives, missed targets, and identity switches.
        \item[IDF1:] Identity F1 (IDF1) score measuring identity preservation through the ratio of correctly identified detections over the average number of ground truth and computed detections.
        \item[MT:] Mostly tracked (MT) ground truth tracks covered for at least 80\% of their length.
        \item[ML:] Mostly lost (ML) ground truth tracks covered for at most 20\% of their length.
        \item[FP:] False positive (FP) bounding boxes not corresponding to any ground truth.
        \item[FN:] False negative (FN) ground truth boxes not covered by any bounding box.
        \item[ID Sw.:] Number of track bounding boxes switching their matched ground truth identity. 
    \end{enumerate}

\section{\methodname}
\label{app_sec:arch_details}

\input{figures/arch_pose2person}
\input{figures/motsynth_gallery}

In~\cref{fig:arch_details}, we show the detailed architecture for \netone and \nettwo. Both networks are trained separately from each other.

\noindent{\bf Pose2Person.} It uses SPADE layers as in~\cite{DBLP:conf/cvpr/Park0WZ19}, and takes as input an identity vector and pose information.
The identity vector is encoded as one-hot vector with the number of the identity we intend to transfer from MOTSynth.
The selected subset of MOTSynth~\cite{motsynth} identities which was used to train the~\netone is visualized in~\cref{fig:motsynth_gallery}.
The pose input is a concatenation of the instance mask and the body joints map. The map of body joints is drawn based only on the common joints between MOTSynth and COCO joint keypoint models.

We train the \netone for $60$ epochs with the Adam optimizer \cite{DBLP:conf/iclr/Kingma14} and a learning rate of $1e-4$.
The Adam beta hyperparameters $\beta_1$ and $\beta_2$ are set to $0.5$ and $0.9$, respectively. 
We train the network for two days in a single GPU and scale input images to $256 \times 128$.

\noindent{\bf Person2Scene.} This network uses a combination of residual blocks. \textit{ResBlockDown} and \textit{ResBlockUp} refer to residual block with downsampling and upsampling, respectively. The output of each decoder block is the level of Laplacian pyramid.
Only the smallest level of the Laplacian pyramid is the low pass representation obtained from computing the Gaussian pyramid of the input image.
We collapse the Laplacian pyramid using upsampling and sum operations on the low pass and output images.

We train \nettwo similarly to \netone, but on $256 \times 256$ image patches with cut out pedestrians. The patch resolution is not constrained by bounding box aspect ratio (as in \netone), so we chose to crop square patches.  Image patches are cropped from random positions in each image in the dataset. During training, we apply sharpness and blur augmentations to the input image.

% \section{MOTSynth gallery design}
% \noindent \textbf{MOTSynth gallery design.}

% \noindent \textbf{Qualitative de-identification results.}

\input{tables/face_anony}
\noindent \textbf{Face de-identification.} 
To compare our work with face de-identification, we checked a blurring and CIAGAN baseline.
For a pedestrian dataset like MOT17, the face landmark/segmentation predictions required for CIAGAN are highly insufficient (see~\cref{tab:face_anony}).
This supports our focus on full-body de-identification for datasets of this kind.

MOT17 does not have GT for face bounding boxes and automatic face detection is not very robust in such a low resolution pedestrian setting. Hence we decided to use the top part of body segmentation masks as our face region. 
To blur face regions, we apply \textit{blur} to the 1/6 part of every input mask from the top.

As shown in the Table on the right, blurring the top part only achieves a deID score close to the original unanonymized data.
More importantly, the downstream task performance also suffers severely, e.g., 59.4 vs 65.3 AP on object detection.
Blurring the top part of the mask neither provides the de-identification properties nor the downstream task performance required for pedestrian dataset generation.

\noindent \textbf{SMPL.}
As explained in the main paper, SMPL model can be fitted to a given set of 2D keypoints and used as an input information. It potentially could provide a full and an unambigious pose for each pedestrian.
For training \netone we use the GT set of 2D keypoints in the MOTSyn dataset, while inference in real dataset uses a predicted set of keypoints.
We show examples in~\cref{fig:smpl_fit}.
However, even using GT keypoints for synthetic pedestrians, SMPL model did not fully fit a required pedestrian silhouette and introduced small errors (as seen for the second pedestrian leg in MOTSyn). 
Real dataset has the same problems but also if keypoints are not fully detected it can lead to strange fitting results as seen for the rightmost pedestrian in~\cref{fig:smpl_fit}.
For inference in \netone, we fitted SMPL only for pedestrians with most of the detected keypoints. For all other pedestrians, we gave blank images for the SMPL part of the input.
% While conceptually promising, the 3D model input gave no additional improvement for detection. In fact, the de- and reID performance got worse. This is most likely due to noise and errors in the predicted keypoints exacerbated by the 3D model. We leave the exploration of additional inputs, e.g., a SMPL version more robust to unreliable keypoints, for future research.

\input{figures/smpl_fig}

\section{\methodname17}
\label{app_sec:AnonyMOT17}

\subsection{Dataset details}

% \noindent \textbf{Synthetic data.}
% The selected subset of MOTSynth~\cite{motsynth} identities which was used to train the~\netone is visualized in~\cref{fig:motsynth_gallery}.
% %
% For the de-identification of MOT17~\cite{MOT16}, we map each real tracking identity to a synthetic one from MOTSynth.
% %
% To de-identify a specific tracking identity, the \netone receives its corresponding MOTSynth identity vector and frame-wise poses consisting of instance masks and keypoints (see~\cref{fig:arch_details}).
% %
% The de-identification is applied on a frame-by-frame basis, processing each frame with our pipeline independently.
%

% \noindent \textbf{\methodname17.}
%
% While the \netone is trained with ground truth synthetic inputs, we rely on predicted masks and joints for the de-identification of MOT17 as it only provides ground truth bounding boxes.
%
% We obtain the predicted pose information by applying a Mask and Keypoint R-CNN, respectively. 
%
% The mask and joint quality directly impacts the generation quality.
%
% However, the MOTS20~\cite{MOTS} dataset provides ground truth masks for a subset of sequences and objects in MOT17.
%
% We therefore map and replace predicted MOT17 masks with available MOTS20~\cite{MOTS} masks.
%

For~\cref{sec:experiments} of the main paper, we evaluate all experiments with a 7-fold split on the 7 MOT17~\cite{MOT16} training sequences, \ie, each validation set contains a single sequence.
We pre-train our models on the ImageNet~\cite{ILSVRC15} dataset or specifically mention if otherwise.
We analyse the applicability of \methodname for the tasks of de-/re-identification, object detection, and multi-object tracking and train each split with the same hyperparameters.
We design the number of epochs for each task such that every split has converged and started to overfit.
%
%The number of epochs mentioned for each task below are designed such that each split has converged and started to overfit. \ili{passive voice :S}
%
We evaluate the results based on the validation metrics averaged over all splits.
%The evaluated results are validation metrics averaged over all splits. \ili{passive, plus not understandable}
%
In particular, we report the results from the epoch which yields the overall best averaged metric and not the average of the best epoch for each individual split. 
Furthermore, this evaluation allows us to estimate the optimal number of training epochs for the final test set benchmark submissions in~\cref{subsec:benchmark}.

\noindent{\bf Input pose generation.}
% \subsection{MOT17 test set generalization}
%
While the \netone is trained with ground truth inputs, we rely on predicted masks and joints for the de-identification of MOT17 as it only provides ground truth bounding boxes.
We obtain the predicted pose information by applying a Mask and Keypoint R-CNN, respectively. 
The mask and joint quality directly impacts the generation quality.
However, the MOTS20~\cite{MOTS} dataset provides ground truth masks for a subset of sequences and objects in MOT17.
We therefore map and replace predicted MOT17 masks with available MOTS20~\cite{MOTS} masks.
For the input poses, we predict instance masks and keypoints for each MOT17 ground truth box with visibility larger than zero.
To this end, we apply a Keypoint and Mask R-CNN with a strong ResNeXt-152~\cite{Xie2016} backbone from the Detectron2~\cite{wu2019detectron2} library.
To further improve the input pose quality, we replace predicted masks with MOTS20~\cite{MOTS} ground truth masks if available.
MOTS20 only provides masks for large objects and a subset of the 7 training sequences.
Unfortunately, MOT17 and MOTS20 do not share consistent tracking identities.
Therefore, we manually compute a matching between the two sets of tracks based on maximal intersection-over-union aggregated over the sequence.

\input{tables/pred_vs_gt_masks}
\noindent \textbf{Predicted vs ground-truth masks.}
Furthermore, we want to demonstrate the robustness of our method to insufficient/predicted input poses.
In~\cref{tab:pred_vs_gt_masks}, we compare the downstream task performance of a dataset de-identified either only with ground-truth or predicted Mask R-CNN \cite{he2017mask} masks. 
Since ground truth is only provided for a subset of objects, the deID performance improves by around 2 points for the more complete set of predicted masks.
However, the reID and detection results suffer from predicted input masks.
We argue that for the de-identification of a new dataset it is reasonable to expect ground truth masks and avoid insufficient inputs for the generation of anonymous identities.
% first annotate the real dataset, then de-identify it with our method before releasing it to the public.
%
% The goal of our method is to de-identify existing or new datasets which can be expected to have sufficient object annotations.

\subsection{MOT17 test set generalization}
\label{app_sec:test_set_generalization}

% As mentioned in\pageref{subsec:benchmark}
As mentioned in~\cref{subsec:benchmark} of the main paper, the MOT17-\{02, 04, 05, 09, 10, 11, 13\} train and MOT17-\{01, 03, 06, 07, 08, 12, 14\} test sequences are not fully unique:
\begin{itemize}
\item MO17-02 (train) and MO17-01 (test) depict the same scene but at different times and camera angles.
\item MOT17-14 (train) and MOT17-13 (test): both taken from a bus and move through very similar street views.
\item MOT17-04 (train) and MOT17-03 (test): these sequences represent the strongest overlap between train and test.
They show the exact same scene from the same view point captured with a small time delay which results in some pedestrians appearing in both.
\end{itemize}

These similarities between the MOT17 train and test set have direct consequences on the generalization and potentially allow models to benefit from a certain degree of overfitting to the training sequences.
However, capitalizing on these similarities is not possible if the training sequences are de-identified.
While \methodname17 achieves results on par with the original MOT17 for our cross validated object detection results presented in~\cref{tab:syn2real} of the main paper, we lack behind in generalization to the test set.
This is mainly because there are no similarities between training sequences, hence, there is no benefit from overfitting during the cross-validation experiments.

In~\cref{tab:mot17det_test_frcnn_per_seq}, we repeat the MOT17Det test set results from the main paper and show a detailed per sequence comparison.
Fine-tuning the model on our \methodname17 dataset results in similar Average Precision (AP) values except for MOT17-03 and MOT17-14.
Both sequences have very similar counterparts in the training set.
To further demonstrate our analysis, we show results for models \textit{not} trained on MOT17-04, where indeed the overall AP gap is significantly reduced.
Since most multi-object tracking methods follow the common tracking-by-detection paradigm, a similar per-sequence analysis would allow for similar conclusions: While MOT17 fails to accurately demonstrate its potential, \methodname17 actually provides sufficient training data for re-identification, detection, and tracking.

\subsection{Qualitative de-identification results.} 
\label{app_sec:qualitative}
In~\cref{fig:qualitative_pose2person}, we illustrate additional qualitative results of our method including the original identity, input pose and resulting de-identification.
For the sake of completeness, we furthermore show some example frames from every \mbox{\methodname17} sequence in~\cref{fig:frame_gallery}.

\noindent \textbf{Failure cases.}
Our de-identification primarily relies on proper instance masks. 
Poorly estimated masks lead to worse synthesis as seen in~\cref{fig:failures_pose2person}. For example, columns 1 and 2 show masks that do not properly outline the body parts of the person and suffer from gaps inside. 
Extreme cases where a person is moving beyond the frame add additional complications for proper synthesis and joint estimations, as shown in columns 3 and 4.
Another common failing is the ambiguity of silhouettes and body joints. Columns 6,7, and 8 show examples where positions of the arms and legs are not easily discernible, hence are not properly generated. 
Finally, as shown in columns 1, 2, 3 and 7, our method does not consider illumination, motion blur and other details that make the de-identified foreground stick out from the background. Such unrealistic adaptations influence visual perception, but it is not clear if they also affect the training of deep learning models. 

\input{tables/mot17det_test_frcnn_per_seq}
\input{figures/frame_gallery}
\begin{figure*}
\begin{center}
\includegraphics[width=0.65\textwidth, trim={0px 0px 210px 0px}, clip]{figures/supp_qualitat2.pdf}
\end{center}
   \caption{
   \textbf{Qualitative results} and input poses of our AnonyMOT anonymization method.
   In the first row we show the original images from different times identities and sequences.
   The second row shows their respective pose information used as an input to \netone.
   The third row shows the blending and adaption with our \nettwo into the given scene.
   }
\label{fig:qualitative_pose2person}
\end{figure*}
\input{figures/failure_pose2person}
